# Supplementary material for: A polyconvex transversely-isotropic invariant-based formulation for electro-mechanics: stability, minimisers and computational implementation
Source: arXiv:2201.05095 source file (2022-01-11)
Supplement: Supplementary file 1 [file appendix.tex]

\begin{appendices}
\section{Stress and stiffness}
The first Piola-Kirchhoff stress can be written as
\begin{eqnarray}
\nonumber
\bm{P} &=& C_1 \frac{\partial \bar{I}_1}{\partial\bm{F}} + \frac{\partial U(J)}{\partial\bm{F}}+ \frac{1}{J\varepsilon_m}\frac{\partial I_7}{\partial\bm{F}} - \frac{I_7}{J^2\varepsilon_m}\cof\bm{F} + C_m(I_4-1) \frac{\partial I_4}{\partial\bm{F}} + \frac{2I_{10}}{J\varepsilon_f}\frac{\partial I_{10}}{\partial \bm{F}} - \frac{I^2_{10}}{J^2\varepsilon_f}\cof \bm{F}
\\
\bm{E}_0 &=& \frac{1}{J\varepsilon_m}\frac{\partial I_7}{\partial\bm{D}_0} + \frac{1}{J\varepsilon_f}\frac{\partial I_{10}}{\partial\bm{D}_0}
\end{eqnarray}

\begin{eqnarray}
\frac{\partial F_{om}F_{on}}{\partial F_{pq}} = \delta_{op}\delta_{mq}F_{on} + \delta_{op}\delta_{nq}F_{om} = F_{pn}\delta_{mq}+F_{pm}\delta_{nq}
\\
\left.\frac{\partial F_{om}F_{on}}{\partial F_{pq}}\right\vert_{\bm{F}=\bm{I}} = \delta_{op}\delta_{mq}F_{on} + \delta_{op}\delta_{nq}F_{om} = \delta_{pn}\delta_{mq}+\delta_{pm}\delta_{nq}
\end{eqnarray}

\begin{eqnarray}
 \frac{\partial \bar{I}_1}{\partial\bm{F}} &=& 2 J^{-2/3}\bm{F} - \frac{2}{3}\bar{I}_1\bm{F}^{-T} \quad \left. \frac{\partial \bar{I}_1}{\partial\bm{F}}\right\vert_{\bm{F}=\bm{I},\bm{D}_0 = \bm{0}}  = \bm{0}
 \\
  \frac{\partial \bar{I}_2}{\partial\bm{F}} &=& J^{-4/3}\bm{F}\bm{\times} -\frac{4}{3}\bar{I}_2\bm{F}^{-T}  \quad \left. \frac{\partial \bar{I}_2}{\partial\bm{F}}\right\vert_{\bm{F}=\bm{I},\bm{D}_0 = \bm{0}}  = \bm{0}
 \\
 \frac{\partial I_3}{\partial\bm{F}} &=& 2J\cof\bm{F}  \quad \left. \frac{\partial \bar{I}_3}{\partial\bm{F}}\right\vert_{\bm{F}=\bm{I},\bm{D}_0 = \bm{0}}  = 2
 \\
 \frac{\partial I_4}{\partial \bm{F}} &=&\frac{\partial I_4}{\partial \bm{C}}:\frac{\partial \bm{C}}{\partial\bm{F}} =  \bm{N}\otimes\bm{N}:\frac{\partial \bm{C}}{\partial\bm{F}} = 
 2\bm{F}\bm{N}\otimes\bm{N} \quad \left. \frac{\partial {I}_4}{\partial\bm{F}}\right\vert_{\bm{F}=\bm{I},\bm{D}_0 = \bm{0}}  = 2\bm{N}\otimes\bm{N} 
\\
 \frac{\partial I_5}{\partial \bm{F}} &=&\frac{\partial I_5}{\partial \bm{C}}:\frac{\partial \bm{C}}{\partial\bm{F}} =  (\bm{N}\otimes\bm{N})\bm{\times}\bm{C}:\frac{\partial \bm{C}}{\partial\bm{F}} = 
 2\bm{F}\bm{N}\otimes\bm{N} \quad \left. \frac{\partial {I}_4}{\partial\bm{F}}\right\vert_{\bm{F}=\bm{I},\bm{D}_0 = \bm{0}}  = 2\bm{N}\otimes\bm{N}
 \\
 \frac{\partial I_6}{\partial\bm{F}} &=& \bm{0} \quad \left. \frac{\partial {I}_6}{\partial\bm{F}}\right\vert_{\bm{F}=\bm{I},\bm{D}_0 = \bm{0}}  = \bm{0}
 \\
 \frac{\partial I_7}{\partial\bm{F}} &=& \frac{\partial I_7}{\partial\bm{C}}\frac{\partial \bm{C}}{\partial\bm{F}} =(\bm{D}_0\otimes\bm{D}_0):\frac{\partial \bm{C}}{\partial\bm{F}} = 2\bm{F}\bm{D}_0\otimes\bm{D}_0\quad \left. \frac{\partial {I}_7}{\partial\bm{F}}\right\vert_{\bm{F}=\bm{I},\bm{D}_0 = \bm{0}}  = \bm{0}
 \\
 \frac{\partial I^2_{10}}{\partial \bm{F}} &=&\frac{\partial I^2_{10}}{\partial \bm{C}}:\frac{\partial \bm{C}}{\partial\bm{F}} =  \frac{2I_{10}}{2}\left(\bm{N}\otimes\bm{D}_0 + \bm{D}_0\otimes\bm{N} \right):\frac{\partial \bm{C}}{\partial\bm{F}} =2I_{10}(\bm{F}\bm{N}\otimes\bm{D}_0 + \bm{F}\bm{D}_0\otimes\bm{N})
 \\
  \left. \frac{\partial {I}^2_{10}}{\partial\bm{F}}\right\vert_{\bm{F}=\bm{I},\bm{D}_0 = \bm{0}}  &=& \bm{0}
 \\
 \frac{\partial I_7}{\partial\bm{D}_0} &=& 2\bm{C}\cdot\bm{D}_0
 \quad \left. \frac{\partial {I}_7}{\partial\bm{D}_0}\right\vert_{\bm{F}=\bm{I},\bm{D}_0 = \bm{0}}  = \bm{0}
 \\
 \frac{\partial I^2_{10}}{\partial\bm{D}_0} &=& 2I_{10}\bm{N}\cdot\bm{C}
 \quad \left. \frac{\partial {I}^2_{10}}{\partial\bm{D}_0}\right\vert_{\bm{F}=\bm{I},\bm{D}_0 = \bm{0}}  = \bm{0}
\end{eqnarray}
Stiffness tensors:
\begin{eqnarray}
\frac{\partial e}{\partial \bm{F}\partial\bm{F}} &=& C_1 \frac{\partial^2 \bar{I}_1}{\partial\bm{F}\partial\bm{F}} + \frac{\partial^2 U(J)}{\partial\bm{F}\partial\bm{F}}+ \frac{1}{J\varepsilon_m}\frac{\partial^2 I_7}{\partial\bm{F}\partial\bm{F}} - \frac{1}{J^2\varepsilon_m}\left(\cof\bm{F}\otimes\frac{\partial I_7}{\partial \bm{F}} + \frac{\partial I_7}{\partial \bm{F}} \otimes\cof\bm{F}  \right) +
\\
&+& 2\frac{I_7}{J^3\varepsilon_m}\cof \bm{F}\otimes\cof \bm{F} - \frac{I_7}{\varepsilon_mJ^2}\bm{F}\bm{\times} +  C_m(I_4-1) \frac{\partial^2 I_4}{\partial\bm{F}\partial\bm{F}}  + C_m \frac{\partial I_4}{\partial \bm{F}}\otimes\frac{\partial I_4}{\partial\bm{F}} +
\\
&+&   \frac{2}{\varepsilon_fJ}\left(\frac{\partial I_{10}}{\partial \bm{F}}\otimes\frac{\partial I_{10}}{\partial \bm{F}} + I_{10}\frac{\partial^2 I_{10}}{\partial \bm{F}\partial \bm{F}}\right)
-\frac{2I_{10}}{J^2\varepsilon_f}\left(\frac{\partial I_{10}}{\partial \bm{F}}\otimes \cof \bm{F} + \cof \bm{F} \otimes \frac{\partial I_{10}}{\partial \bm{F}}\right) +  
\\
&+&2\frac{I^2_{10}}{J^3\varepsilon_f}\cof \bm{F}\otimes \cof \bm{F}
-\frac{I^2_{10}}{J^2\varepsilon_f}\bm{F}\bm{\times}
\\
\frac{\partial e}{\partial \bm{D}_0\partial\bm{D}_0} &=& \frac{1}{J\varepsilon_m}\frac{\partial^2 I_7}{\partial\bm{D}_0\partial\bm{D}_0} + \frac{2I_{10}}{J\varepsilon_f}\frac{\partial^2 I_{10}}{\partial\bm{D}_0\partial\bm{D}_0} +\frac{2}{J\varepsilon_f}\frac{\partial I_{10}}{\partial\bm{D}_0}\otimes\frac{\partial I_{10}}{\partial\bm{D}_0}
\\
\nonumber
\frac{\partial e}{\partial \bm{D}_0\partial\bm{F}} &=& \frac{1}{J\varepsilon_m}\frac{\partial^2 I_7}{\partial\bm{D}_0\partial\bm{F}} + \frac{2I_{10}}{J\varepsilon_f}\frac{\partial^2 I_{10}}{\partial\bm{D}_0\partial\bm{F}} + \frac{2}{J\varepsilon_f}\frac{\partial I_{10}}{\partial\bm{D}_0}\otimes\frac{\partial I_{10}}{\partial\bm{F}} - \frac{1}{J^2\varepsilon_m}\frac{\partial I_7}{\partial\bm{D}_0}\otimes\cof\bm{F} - \frac{2I_{10}}{J\varepsilon_f}\frac{\partial I_{10}}{\partial\bm{D}_0}\otimes\cof\bm{F}
\\
\nonumber
\frac{\partial e}{\partial\bm{F} \partial\bm{D}_0} &=& \frac{1}{J\varepsilon_m}\frac{\partial^2 I_7}{\partial\bm{F}\partial\bm{D}_0} + \frac{2I_{10}}{J\varepsilon_f}\frac{\partial^2 I_{10}}{\partial\bm{F}\partial\bm{D}_0} + \frac{2}{J\varepsilon_f}\frac{\partial I_{10}}{\partial\bm{F}}\otimes\frac{\partial I_{10}}{\partial\bm{D}_0} - \frac{1}{J^2\varepsilon_m}\cof\bm{F}\otimes\frac{\partial I_7}{\partial\bm{D}_0}-\frac{2I_{10}}{J\varepsilon_f}\cof\bm{F}\otimes\frac{\partial I_{10}}{\partial\bm{D}_0}
\end{eqnarray}
with
\begin{eqnarray}
 \frac{\partial^2 I_4}{\partial \bm{F}\partial \bm{F}} &=& 2\bm{\delta}\underline{\otimes}(\bm{N}\otimes\bm{N})
\\
 \frac{\partial^2 I_7}{\partial\bm{F}\partial\bm{F}} &=& 2\bm{\delta}\underline{\otimes}(\bm{D}_0\otimes\bm{D}_0)
 \\
 \frac{\partial^2 I_{10}}{\partial \bm{F}\partial \bm{F}} &=&
 \bm{\delta}\underline{\otimes}(\bm{D}_0\otimes\bm{N}) + (\bm{N}\otimes\bm{D}_0)\overline{\otimes}\bm{\delta}
 \\
 \frac{\partial^2 I_7}{\partial\bm{D}_0\partial\bm{D}_0} &=& 2\bm{C}
 \\
 \frac{\partial^2 I_{10}}{\partial\bm{D}_0 \partial\bm{D}_0} &=& \bm{0}
 \\
 \frac{\partial^2 I_7}{\partial\bm{F}\partial\bm{D}_0} &=& 2(F_{in}D_n\delta_{kj} + F_{ik}D_j)
 \\
 \frac{\partial^2 I_{10}}{\partial\bm{D}_0\partial\bm{F}_0} &=& F_{iq}N_q\delta_{jk} + N_iF_{jk}
\end{eqnarray}
%%%%%%%%%%%%%%%%%%%%%%%%%%%%%%%%%%%5

\section{Magneto-mechanics}\label{sec:Appendix_Danas}
{\mh In this appendix, we briefly comment on the applicability of the presented analysis towards magneto-mechanics. In the magnetic case, the Lagrangian electric displacement is  replaced by the Lagrangian magnetic induction $\bm{B}_0$ which evolution is governed by the first law of magnetostatics as
\begin{eqnarray}
\div\bm{B}_0 = 0 
\end{eqnarray}
Therefore, the condition of polyconvexity for magneto-mechanics is of the same form as for the electro-mechanics; namely, function $W(\bm{F}, \bm{B}_0):\R^{3\times 3}\times \R^{3}\times \R^{3}\to\R\cup\{+\infty\}$ is polyconvex if  there exists a convex and a lower semicontinuous function $g_m :\mathbb{R}^{3\times3}\times\mathbb{R}^{3\times3}\times\mathbb{R}\times\mathbb{R}^3\times\mathbb{R}^3\times\mathbb{R}^3\times\mathbb{R}^3 \to \mathbb{R}\cup\{+\infty\}$ such that
\begin{align}\label{polyconvexity_em}
W(\bm{F}, \bm{B}_0) = g_m(\bm{F}, {\cof}\bm{F}, \det \bm{F}, \bm{B}_0, \bm{F}\bm{B}_0)\ .
\end{align}
Moreover, invariants for a transversely isotropic magneto-elastic material are the same as for the electro-mechanics just with $\bm{D}_0$ replaced by $\bm{B}_0$. Therefore, the whole analysis of polyconvexity presented in this work is directly transferable to magneto-elastic materials. 
}
\begin{eqnarray}
\Psi_{sat} = \Psi + \frac{G}{2}\left(\left[-0.1216\left(\frac{I_6}{I_7}-\frac{I_9}{I_7}\right)+0.167\left(\frac{I_6}{I_8}-\frac{I_9}{I_8}\right)\right]\left(\frac{I_6}{M_s^2}\right)^2\right)\left(\frac{1}{2}{\rm ln}\left[1-\left(\frac{I_6}{M_s^2}\right)^2\right] + \frac{I_6}{M_s^2}\tanh^{-1}\left(\frac{I_6}{M_s^2}\right)\right)
\end{eqnarray}
\end{appendices}
