# Supplementary material for: A polyconvex transversely-isotropic invariant-based formulation for electro-mechanics: stability, minimisers and computational implementation
Source: arXiv:2201.05095 source file (2022-01-11)
Supplement: Supplementary file 2 [file Appendix_jump_conditions.tex]

Consider a travelling discontinuity within the electroactive material, moving at speed $c$ and defined by a normal vector $\vect{V}$ separating states $(\bullet)^a$ and $(\bullet)^b$,  where $\llbracket\bullet\rrbracket =(\bullet)^a-(\bullet)^b$ denotes the jump across the interface and $(\bullet)^{{\text{Av}}}=1/2((\bullet)^a+(\bullet)^b)$ the average state. The jump or Rankine-Hugoniot conditions for the combined set of Cauchy-Maxwell equations are given by
\begin{subequations}
\begin{align}
-c\llbracket  \vect{F}\rrbracket&= \llbracket \vect{v}\rrbracket \otimes \vect{V};\label{eqn:jump1}\\
-c\rho\llbracket  \vect{v}\rrbracket&= \llbracket \vect{P}\rrbracket  \vect{V};\label{eqn:jump2}\\
-c\llbracket \vect{B}_0\rrbracket&= \llbracket \vect{E}_0\rrbracket \times \vect{V};\label{eqn:jump3}\\
c\llbracket  \vect{D}_0\rrbracket&= \llbracket \vect{H}_0\rrbracket \times \vect{V};\label{eqn:jump4}\\
-c\llbracket e +1/2\rho \vect{v}\cdot \vect{v}\rrbracket&=\llbracket\vect{v}\cdot \vect{P} \rrbracket \cdot \vect{V} -\llbracket \vect{E}_0 \times \vect{H}_0\rrbracket \cdot \vect{V},\label{eqn:jump5}
\end{align}
\end{subequations}
where, in addition to previoulsy defined fields, $\rho$, $\vect{v}$, $\vect{B}_0$ and $\vect{H}_0$ denote the density of the material per unit undeformed volume, the velocity, the magnetic induction vector and the magnetic field, respectively. Substitution of \eqref{eqn:jump1}-\eqref{eqn:jump4} into \eqref{eqn:jump5} renders
\begin{equation} \label{eqn:jump5b}
\begin{aligned}
\llbracket e \rrbracket&=\vect{P}^{\text{Av}}:\llbracket\vect{F} \rrbracket + \vect{E}_0^{\text{Av}}\cdot \llbracket\vect{D}_0 \rrbracket +\vect{H}_0^{\text{Av}}\cdot\llbracket\vect{B}_0 \rrbracket,
\end{aligned}
\end{equation}
which, by re-defining $(\bullet)^{\text{Av}}=(\bullet)+\llbracket \bullet \rrbracket/2$, can be rewritten as
\begin{equation} \label{eqn:jump5c}
\begin{aligned}
\llbracket e \rrbracket-\vect{P}:\llbracket\vect{F} \rrbracket - \vect{E}_0\cdot\llbracket\vect{D}_0 \rrbracket -\vect{H}_0\cdot\llbracket\vect{B}_0 \rrbracket &= \llbracket\vect{P}\rrbracket:\llbracket\vect{F} \rrbracket + \llbracket\vect{E}_0\rrbracket\cdot\llbracket\vect{D}_0 \rrbracket +\llbracket\vect{H}_0\rrbracket\cdot\llbracket\vect{B}_0 \rrbracket.
\end{aligned}
\end{equation}

For the simpler case when magnetic effects are neglected (i.e. $\llbracket \vect{B}_0 \rrbracket \approx \vect{0}$) the last term on both sides of above equation \eqref{eqn:jump5c} can be neglected. Moreover, notice that the term $\llbracket\vect{E}_0\rrbracket\cdot\llbracket\vect{D}_0 \rrbracket \approx \vect{0}$ as $\vect{E}_0$ can thus only jump tangentially across the discontinuity (refer to \eqref{eqn:jump3}) whilst $\vect{D}_0$ can only jump along $\vect{V}$ (refer to \eqref{eqn:jump4}), that is, $\llbracket\vect{D}_0 \rrbracket=\vect{V}_{\perp}$, $\vect{V}\cdot \vect{V}_{\perp}=0$. Thus, we arrive at the simpler equation 
\begin{equation} \label{eqn:jump5d}
\begin{aligned}
\llbracket e \rrbracket-\vect{P}:\llbracket\vect{F} \rrbracket - \vect{E}_0\cdot \vect{V}_{\perp}   &= \llbracket\vect{P}\rrbracket:\llbracket\vect{F} \rrbracket.
\end{aligned}
\end{equation}

Redefining $-\llbracket  \vect{v}\rrbracket/c=\vect{u}$, that is $\llbracket\vect{F}\rrbracket=\vect{u} \otimes \vect{V}$, and making use of \eqref{eqn:jump1} and \eqref{eqn:jump2}, it is straightforward to show that $\llbracket\vect{P}\rrbracket:\llbracket\vect{F} \rrbracket=\rho c^2 \vect{u}\cdot \vect{u}$, which finally gives
\begin{equation} \label{eqn:jump5e}
\begin{aligned}
\llbracket e \rrbracket-\vect{P}:(\vect{u} \otimes \vect{V}) - \vect{E}_0\cdot \vect{V}_{\perp}   &= \rho c^2 \vect{u}\cdot \vect{u}\geq 0,
\end{aligned}
\end{equation}
which can be equivalently written as
\begin{equation}\label{eqn:rank-1}
e(\vect{F}+\vect{u}\otimes \vect{V},\vect{D}_0 + \vect{V}_{\perp})-e(\vect{F},\vect{D}_0)-\partial_{\vect{F}}e :(\vect{u}\otimes \vect{V})-\partial_{\vect{D}_0}e \cdot \vect{V}_{\perp}\geq 0.
\end{equation}

Notice that above inequality \eqref{eqn:rank-1} holds for an energy density $e(\boldsymbol{\mathcal{U}})$ defined as rank-one convex (refer to equation \eqref{eqn:rank1_der1}).
